# Supplementary material for: Anomalous conductances in an ultracold quantum wire
Source: arXiv:1607.02509 ancillary file (2016-07-08)
Supplement: Supplementary file 1 [file NSN_Supplementary_1_9.pdf]

# Supplementary Material for Anomalous conductances in an ultracold quantum wire

M. Kanász-Nagy[1], L. Glazman[2], T. Esslinger[3], and E. A. Demler[1]
[1]*Department of Physics, Harvard University, Cambridge, MA 02138, U.S.A.*
[2]*Department of Physics, Yale University, New Haven, CT 06520, U.S.A. and*
[3]*Department of Physics, ETH Zurich, 8093 Zurich, Switzerland*

## I. HAMILTONIAN

We determine the superconducting profile inside the elliptic constriction within the local density approximation (LDA). Assuming harmonic confinement in the $x$ and $z$ transverse directions, the kinetic and interacting part of the local Hamiltonian are given by

$$H_{\text{kin}} = \int d^3r \sum_{\sigma=\uparrow,\downarrow} \phi^\dagger_\sigma(\mathbf{r}) \left( -\frac{\hbar^2\Delta}{2m} + \frac{m}{2}\left(\omega_x^2 x^2 + \omega_z^2 z^2\right) - \mu_\sigma - V_g \right) \phi_\sigma(\mathbf{r}), \tag{S1}$$

$$H_{\text{int}} = g \int d^3r\, \phi^\dagger_\uparrow(\mathbf{r})\phi^\dagger_\downarrow(\mathbf{r})\phi_\downarrow(\mathbf{r})\phi_\uparrow(\mathbf{r}), \tag{S2}$$

where $\omega_x$ and $\omega_z$ denote the local values of the trapping frequencies, whereas $V_g$ stands for that of the gate potential. In equilibrium, the chemical potentials $\mu_\sigma$ are constant across the constriction, and they are set by the leads. The bare coupling constant $g$ is related to the scattering lengths, as we discuss in Sec. III A. We decompose the fermionic fields $\phi_\sigma(\mathbf{r})$ in terms of the eigenmodes of the transverse confining potential

$$\phi_\sigma(\mathbf{r}) \equiv \frac{1}{\sqrt{L_y}} \sum_{\mathbf{n}=(n_x,n_z)} \sum_q e^{iqy}\, \varphi_{n_x}(x)\varphi_{n_z}(z)\, a_{\mathbf{n},\sigma,q},$$

where $\mathbf{n} = (n_x, n_z)$ denotes the transverse harmonic oscillator quantum numbers, and $L_y$ is the length of the system. $\varphi_{n_{x(z)}}$ stands for the harmonic oscillator wave functions of oscillator length $l_{x(z)}$. We rewrite the Hamiltonian in terms of these transverse modes as

$$H_{\text{kin}} = \sum_{\sigma=\uparrow,\downarrow} \sum_{\mathbf{n},q} \xi_{\mathbf{n},\sigma,q}\, a^\dagger_{\mathbf{n},\sigma,q}\, a_{\mathbf{n},\sigma,q}$$

$$H_{\text{int}} = \frac{g}{L_y} \sum_{\mathbf{n}_1\mathbf{n}_2\mathbf{n}_3\mathbf{n}_4} \sum_{k,k',q} \langle\langle \mathbf{n}_1\mathbf{n}_2 || \mathbf{n}_3\mathbf{n}_4 \rangle\rangle\, a^\dagger_{\mathbf{n}_1,\uparrow,k+q} a^\dagger_{\mathbf{n}_2,\downarrow,k'-q} a_{\mathbf{n}_3,\downarrow,k'} a_{\mathbf{n}_4,\uparrow,k},$$

with the single particle energies $\xi_{\mathbf{n},\sigma,q}$ given below Eq. (1) in the main text. The matrix element of the Dirac delta interaction potential with transverse oscillator modes is given by

$$\begin{aligned} \langle\langle \mathbf{n}_1\mathbf{n}_2 || \mathbf{n}_3\mathbf{n}_4 \rangle\rangle \equiv\; & \langle \varphi_{n_{x1}}(x_1), \varphi_{n_{x2}}(x_2)|\, \delta(x_1 - x_2)\, |\varphi_{n_{x3}}(x_2), \varphi_{n_{x4}}(x_1)\rangle \\ & \cdot\; \langle \varphi_{n_{z1}}(z_1), \varphi_{n_{z2}}(z_2)|\, \delta(z_1 - z_2)\, |\varphi_{n_{z3}}(z_2), \varphi_{n_{z4}}(z_1)\rangle\,. \end{aligned} \tag{S3}$$

## II. SUPERCONDUCTING FREE ENERGY

We calculate the superconducting free energy inside the constriction within Bardeen–Cooper–Schrieffer (BCS) theory. Our analysis is an extension of the approach of Ref. 1 that considered BCS mean-field theory in quasi-two-dimensional geometry. As a first step, we transform the Hamiltonian into the basis of relative and center of mass coordinates $(X, Z) = ((x_1 + x_2)/2, (z_1 + z_2)/2)$ and $(\tilde{x}, \tilde{z}) = (x_1 - x_2, z_1 - z_2)$. The associated harmonic oscillator modes can be written as

$$|N_x\rangle \equiv 2^{1/4}\, \varphi_{N_x}\left(\sqrt{2}X\right), \qquad |\nu_x\rangle \equiv \frac{1}{2^{1/4}}\, \varphi_{\nu_x}\left(\tilde{x}/\sqrt{2}\right) \equiv \tilde{\varphi}_{\nu_x}(\tilde{x}),$$

and similarly for the $z$ axis. Within this basis, the interaction matrix element Eq. (S3) is given by

$$\langle\langle \mathbf{n}_1, \mathbf{n}_2 || \mathbf{n}_3, \mathbf{n}_4 \rangle\rangle = \sum_{\mathbf{N}_1,\mathbf{N}_2,\boldsymbol{\nu}_1,\boldsymbol{\nu}_2} \langle \mathbf{n}_1, \mathbf{n}_2 | \mathbf{N}_1, \boldsymbol{\nu}_1\rangle\, \langle \mathbf{N}_2, \boldsymbol{\nu}_2 | \mathbf{n}_3, \mathbf{n}_4\rangle\, \tilde{\varphi}_{\boldsymbol{\nu}_1}(0)\tilde{\varphi}_{\boldsymbol{\nu}_2}(0)\, \delta_{\mathbf{N}_1,\mathbf{N}_2}, \tag{S4}$$

where we introduced the notations $|\mathbf{N}\rangle \equiv |N_x, N_z\rangle$, $|\boldsymbol{\nu}\rangle \equiv |\nu_x, \nu_z\rangle$, and $\tilde{\varphi}_{\boldsymbol{\nu}}(0) \equiv \tilde{\varphi}_{\nu_x}(0)\, \tilde{\varphi}_{\nu_z}(0)$. Since the interaction only depends on the relative coordinates of the colliding atoms, the center of mass quantum number is conserved. Using the orthogonality property of single particle eigenstates, one finds that only those matrix elements $\langle \mathbf{n}_1, \mathbf{n}_2 | \mathbf{N}, \boldsymbol{\nu}\rangle$ are non-zero, for which $\mathbf{n}_1 + \mathbf{n}_2 = \mathbf{N} + \boldsymbol{\nu}$.

We define the dimensionless matrix elements $V^{\mathbf{n}_1\mathbf{n}_2}_{\mathbf{N}} \equiv \sqrt{l_x\, l_z}\, \tilde{\varphi}_{\boldsymbol{\nu}}(0)\, \langle \mathbf{N}\boldsymbol{\nu} | \mathbf{n}_1\mathbf{n}_2\rangle$, where the oscillator mode of transverse motion is given by $\boldsymbol{\nu} \equiv \mathbf{n}_1 + \mathbf{n}_2 - \mathbf{N}$. We rewrite the interaction vertex Eq. (S4) as

$$\langle\langle \mathbf{n}_1\mathbf{n}_2 || \mathbf{n}_3\mathbf{n}_4 \rangle\rangle = \frac{1}{l_x\, l_z} \sum_{\mathbf{N}} (V^\dagger_{\mathbf{N}})^{\mathbf{n}_1\mathbf{n}_2}\, V^{\mathbf{n}_3\mathbf{n}_4}_{\mathbf{N}}. \tag{S5}$$

Using these matrix elements, we express the interaction Hamiltonian in the form

$$H_{\rm int} = \frac{1}{\tilde{g}} \sum_{\mathbf{N},q} \hat{\Delta}^\dagger_{\mathbf{N},q} \hat{\Delta}_{\mathbf{N},q},$$

introducing the operators $\hat{\Delta}_{\mathbf{N},q} \equiv \tilde{g} \sum_{\mathbf{n_3 n_4}} V_{\mathbf{N}}^{\mathbf{n_3 n_4}} \sum_k a_{\mathbf{n}_3,\downarrow,q-k} a_{\mathbf{n}_4,\uparrow,k}$, and the bare coupling $\tilde{g} = g/(L_y l_x l_z)$, which has dimension energy. We introduce separate order parameters for every one of the transverse center of mass channels $N$, but assume that only $q = 0$ acquires non-zero expectation value, $\Delta_{\mathbf{N}} \equiv \langle \hat{\Delta}_{\mathbf{N},q=0} \rangle$. This is analogous to the assumption of the zero momentum pairing for homogeneous superconductors. We decouple the interaction within BCS theory, and arrive at the mean-field Hamiltonian

$$H_{\rm MF} = \sum_{\mathbf{n}_1,\mathbf{n}_2,q} \begin{pmatrix} a^\dagger_{\mathbf{n}_1,\uparrow,q}, a_{\mathbf{n}_1,\downarrow,-q} \end{pmatrix} \begin{pmatrix} \boldsymbol{\xi}_{\uparrow,q} & \boldsymbol{\Delta} \\ \boldsymbol{\Delta}^\dagger & -\boldsymbol{\xi}_{\downarrow,q} \end{pmatrix} \begin{pmatrix} a_{\mathbf{n}_2,\uparrow,q} \\ a^\dagger_{\mathbf{n}_2,\downarrow,-q} \end{pmatrix} + \sum_{\mathbf{n},q} \xi_{\mathbf{n}_1,\downarrow,q} - \sum_{\mathbf{N}} \frac{|\Delta_{\mathbf{N}}|^2}{\tilde{g}}, \tag{S6}$$

with the kinetic and pairing terms given by $\left(\boldsymbol{\xi}_{\sigma,q}\right)_{\mathbf{n}_1\mathbf{n}_2} = \delta_{\mathbf{n}_1\mathbf{n}_2} \xi_{\sigma,\mathbf{n}_1,q}$ and $\boldsymbol{\Delta}_{\mathbf{n}_1\mathbf{n}_2} = \sum_{\mathbf{N}} \Delta_{\mathbf{N}} (V^\dagger_{\mathbf{N}})^{\mathbf{n}_1\mathbf{n}_2}$, respectively.

We diagonalize $H_{\rm MF}$ using the Bogoliubov transformation

$$\begin{pmatrix} \gamma^\dagger_{\uparrow,q} \\ \gamma_{\downarrow,q} \end{pmatrix} = \begin{pmatrix} \mathbf{u}_q & -\mathbf{v}^*_q \\ \mathbf{v}_q & \mathbf{u}^*_q \end{pmatrix} \begin{pmatrix} \mathbf{a}^\dagger_{\uparrow,q} \\ \mathbf{a}_{\downarrow,-q} \end{pmatrix}.$$

where the unitarity of the transformation ensures that operators $\gamma_{\sigma,\mathbf{n},q}$ obey fermionic anti-commutation relations. After the Bogoliubov transformation,

$$\begin{pmatrix} \mathbf{u}_q & -\mathbf{v}^*_q \\ \mathbf{v}_q & \mathbf{u}^*_q \end{pmatrix}^\dagger \begin{pmatrix} \boldsymbol{\xi}_{\uparrow,q} & \boldsymbol{\Delta} \\ \boldsymbol{\Delta}^\dagger & -\boldsymbol{\xi}_{\downarrow,q} \end{pmatrix} \begin{pmatrix} \mathbf{u}_q & -\mathbf{v}^*_q \\ \mathbf{v}_q & \mathbf{u}^*_q \end{pmatrix} = \begin{pmatrix} \mathbf{E}_q & 0 \\ 0 & -\mathbf{E}_q \end{pmatrix} \tag{S7}$$

the Hamiltonian becomes diagonal, $H_{\rm MF} = E_{\rm MF} + \sum_{\mathbf{n},q,\sigma} E_{\mathbf{n},q}\, \gamma^\dagger_{\sigma,\mathbf{n},q} \gamma_{\sigma,\mathbf{n},q}$, with the ground state energy

$$E_{\rm MF} = \sum_{\mathbf{n},q} (\xi_{\downarrow,\mathbf{n},q} - E_{\mathbf{n},q}) - \sum_{\mathbf{N}} \frac{|\Delta_{\mathbf{N}}|^2}{\tilde{g}}. \tag{S8}$$

In order to determine the superconducting order parameters $\Delta_{\mathbf{N}}$ across the constriction, we need to find the minimum of the BCS free energy $F_{MF} = E_{MF} - k_B T \sum_{\mathbf{n},\sigma,q} \log\left(1 + e^{-E_{\mathbf{n}\sigma q}/k_B T}\right)$ with respect to $\Delta_{\mathbf{N}}$, at a finite temperature $T$.

One of the challenges in analyzing equation (S8) is that taken directly with the coupling constant $\tilde{g}$, it is UV divergent. However this divergence should disappear when one uses the Lippmann–Schwinger relation between the microscopic interaction and the scattering length $a$. This is similar to the three dimensional case, where the free energy can be regularized after expressing the bare coupling in terms of the scattering length, $a$ [2]. Details of such regularization procedure for quasi-one dimensional gases are presented in Sec. III. One of the aspects of this analysis is the effect of the confinement potential on the $T$-matrix describing two particle scattering processes. In particular, it describes the well known phenomenon that tighter confinement gives rise to stronger pairing [1]. Thus the constriction can be superconducting even at temperatures where the leads are in the normal phase. This is the key ingredient of our analysis.

## III. CONFINEMENT INDUCED RENORMALIZATION OF INTERACTIONS IN THE TWO-PARTICLE PROBLEM

As has been pointed out by Olshanii [3], and Petrov and Shlyapnikov [4, 5], confining cold atoms into low dimensional structures leads to strong renormalization of their interactions, which can even lead to the so-called confinement induced resonances [6–11]. The effective interaction of atoms within the confined system are characterized by the $T$-matrix describing two particle scattering processes. In this section, we use the vacuum $T$-matrix as a tool to determine the bare coupling $g$ in terms of physically measurable quantities, the scattering length $a$ and the vacuum two-particle bound state energy $E_B$ of the confined system. As we show in Sec. III A, this makes Eq. (S8) divergence-free. The $T$-matrix can be determined using the Bethe–Salpeter equation [12, 13], which takes on a particularly simple form in the vacuum, where only ladder diagrams contribute to the $T$-matrix,

$$T_{\vec{\mathbf{n}},\vec{\mathbf{n}}'}(\omega,\mathbf{q}) = g\,\langle\langle \vec{\mathbf{n}} || \vec{\mathbf{n}}' \rangle\rangle + \sum_{\vec{\mathbf{n}}''} g\,\langle\langle \vec{\mathbf{n}} || \vec{\mathbf{n}}'' \rangle\rangle\, \Pi^{(0)}_{\vec{\mathbf{n}}''}(\omega,\mathbf{q})\, T_{\vec{\mathbf{n}}'',\vec{\mathbf{n}}'}(\omega,\mathbf{q}), \tag{S9}$$

as depicted in Fig. S1. The solid lines stand for vacuum propagators, whereas the dashed lines denote the interaction vertex $g\,\langle\langle\vec{\mathbf{n}}||\vec{\mathbf{n}}'\rangle\rangle$, with $\vec{\mathbf{n}} = (\mathbf{n}_1, \mathbf{n}_2)$ denoting the channel indices of the particle pairs. The polarization operator, corresponding to the pairs of propagators, is defined as [13]

$$\Pi^{(0)}_{(\mathbf{n}_1,\mathbf{n}_2)}(\omega, \mathbf{q}) = \int \frac{dk}{2\pi} \frac{1}{\hbar\omega + i0^+ - \left(\frac{\hbar^2 k^2}{m} + \frac{\hbar^2 q^2}{4m} + \hbar(\mathbf{n}_1 + \mathbf{n}_2)\boldsymbol{\omega}\right)}, \tag{S10}$$

with $\boldsymbol{\omega} = (\omega_x, \omega_z)$.

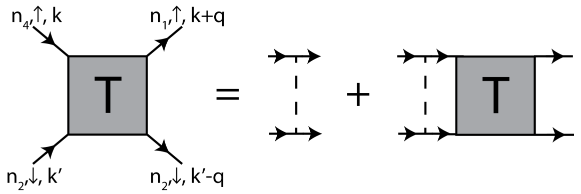


FIG. S1. Bethe–Salpeter equations in the confined system. Solid lines denote vacuum propagators, whereas dashed lines stand for the interaction vertex $g\,\langle\langle \mathbf{n}_1\mathbf{n}_2||\mathbf{n}_3\mathbf{n}_4\rangle\rangle$.

In the two particle problem, parabolic confinement potentials have the special feature of complete separation of center of mass and relative motion. In the basis of center of mass and relative coordinates, the Bethe–Salpeter equation takes a simpler form

$$T^{(0)}_{\mathbf{N}\boldsymbol{\nu};\mathbf{N}'\boldsymbol{\nu}'}(\omega, q) = \sum_{\mathbf{n}_1,\mathbf{n}_2,\mathbf{n}_1',\mathbf{n}_2'} \langle \mathbf{N}, \boldsymbol{\nu}|\mathbf{n}_1, \mathbf{n}_2\rangle\, T^{(0)}_{\mathbf{n}_1,\mathbf{n}_2;\mathbf{n}_1',\mathbf{n}_2'}(\omega, q)\, \langle \mathbf{n}_1', \mathbf{n}_2'|\mathbf{N}', \boldsymbol{\nu}'\rangle\,.$$

Note that in the last equation, the vacuum polarization operator Eq. (S10) depends on the center of mass coordinates only via an energy shift,

$$\Pi^{(0)}_{\mathbf{n}_1,\mathbf{n}_2}(\omega, q) = \Pi^{(0)}_{\mathbf{N}+\boldsymbol{\nu}}(\omega, q) = \Pi^{(0)}_{\boldsymbol{\nu}}(\omega - \mathbf{N}\cdot\boldsymbol{\omega}, q),$$

with $\mathbf{n}_1 + \mathbf{n}_2 = \mathbf{N} + \nu$. We solve the Bethe–Salpeter equation using the following ansatz [13]

$$T^{(0)}_{\mathbf{N}\boldsymbol{\nu};\mathbf{N}'\boldsymbol{\nu}'}(\omega, q) = \delta_{\mathbf{N},\mathbf{N}'}\, \tilde{\varphi}_{\boldsymbol{\nu}}(0)\tilde{\varphi}_{\boldsymbol{\nu}'}(0)\, \mathcal{T}(\omega - \mathbf{N}\cdot\boldsymbol{\omega}, q), \tag{S11}$$

that allows us to express the $T$-matrix in terms of the bare coupling in Eq. (S9)

$$\frac{1}{g} = \frac{1}{\mathcal{T}(\omega, q)} + \sum_{\boldsymbol{\nu}} |\tilde{\varphi}_{\boldsymbol{\nu}}(0)|^2\, \Pi^{(0)}_{\boldsymbol{\nu}}(\omega, q). \tag{S12}$$

### A. Regularization of the bare coupling

Eq. (S12) is UV-divergent as expressed in terms of the bare coupling. To deal with this singularity, we express $g$ in terms of the scattering length $a$, which is related to the $T$-matrix of a three dimensional gas as [13]

$$\frac{4\pi\hbar^2 a}{m} = T^{\mathrm{3D}}(\omega \to 0-, \mathbf{q} = 0). \tag{S13}$$

In the absence of confining potentials, the vacuum Bethe–Salpeter equations take on the simple form

$$T^{\mathrm{3D}}(\omega, \mathbf{q}) = g + g\,\Pi^{\mathrm{3D}}(\omega, \mathbf{q})\, T^{\mathrm{3D}}(\omega, \mathbf{q}), \tag{S14}$$

where the polarization operator is given by

$$\Pi^{\mathrm{3D}}(\omega, \mathbf{q}) = \int \frac{d^3k}{(2\pi)^3} \frac{1}{\hbar\omega + i0^+ - \hbar^2\left(\frac{\mathbf{k}^2}{m} + \frac{\mathbf{q}^2}{4m}\right)}.$$

At negative frequencies, the denominator of this expression is negative, we can thus make use of the integral identity $A^{-1} = -\int_0^\infty d\tau\, e^{\tau A}$, and rewrite it as

$$\Pi^{\rm 3D}(\omega,\mathbf{q}) = -\int_0^\infty d\tau e^{\tau(\hbar\omega+i0^+-\hbar^2\mathbf{q}^2/4m)} \int \frac{d^3k}{(2\pi)^3} e^{-\frac{\tau}{m}\hbar^2\mathbf{k}^2} = -\int_0^\infty d\tau e^{\tau(\hbar\omega+i0^+-\hbar^2\mathbf{q}^2/4m)} \left(\frac{m}{4\pi\hbar^2\tau}\right)^{3/2}.$$

Taking the $\omega \to 0-$ limit, and using Eq. (S13) allows one to express the coupling constant $g$ in terms of the scattering length

$$\frac{1}{g} = \frac{m}{4\pi\hbar^2 a} - \int \frac{d^3k}{(2\pi)^3} \frac{k}{\hbar^2k^2 + i0^+} = \frac{m}{4\pi\hbar^2 a} - \int_0^\infty d\tau \left(\frac{m}{4\pi\hbar^2\tau}\right)^{3/2}. \tag{S15}$$

This expression is equivalent to the first line of Eq. (5) in the main text.

### B. Confinement effects

The $T$-matrix Eq. (S12) of the confined system can thus be written in terms of the scattering length instead of the bare coupling. Although Eqs. (S12) and (S15) are both divergent, their singular parts exactly cancel each other. The $T$-matrix thus becomes regular, as we show in the remaining part of this section, through a somewhat technical derivation. First, we split the summation in Eq. (S12) over transverse harmonic oscillator modes into two parts. Let $\tilde\nu_x$ and $\tilde\nu_z$ be two arbitrary transverse mode indices, such that the motion of the particle pair in the corresponding channels are evanescent, $\hbar\omega + \hbar^2q^2/4m < \hbar\tilde\nu_x, \hbar\tilde\nu_z$. For $\nu_x \le \tilde\nu_x$ and $\nu_z \le \tilde\nu_z$, we represent the polarization operators using the following analytical form

$$\Pi^{(0)}_{\boldsymbol{\nu}}(\omega,q) = \int \frac{dk}{2\pi} \frac{1}{\hbar\omega + i0^+ - \left(\frac{\hbar^2k^2}{m} + \frac{\hbar^2q^2}{4m} + \hbar\boldsymbol{\nu}\cdot\boldsymbol{\omega}\right)} = -i\sqrt{\frac{m/(4\hbar^2)}{\hbar\omega + i0^+ - \left(\frac{\hbar^2q^2}{4m} + \hbar\boldsymbol{\nu}\cdot\boldsymbol{\omega}\right)}}. \tag{S16}$$

In case of all other channels, the denominator of the momentum integral in Eq. (S16) is negative, and we can rewrite the polarization operator as an exponential integral

$$\Pi^{(0)}_{\boldsymbol{\nu}}(\omega,q) = \int_0^\infty d\tau\, e^{\tau\left(\hbar\omega+i0^+-\frac{\hbar^2q^2}{4m}-\hbar\boldsymbol{\nu}\cdot\boldsymbol{\omega}\right)} \int \frac{dk}{2\pi} e^{-\tau\frac{\hbar^2k^2}{m}} = \sqrt{\frac{m}{4\pi\hbar^2}} \int_0^\infty \frac{d\tau}{\sqrt{\tau}}\, e^{\tau\left(\hbar\omega+i0^+-\frac{\hbar^2q^2}{4m}-\hbar\boldsymbol{\nu}\cdot\boldsymbol{\omega}\right)}. \tag{S17}$$

This exponential form allows one to sum up the harmonic oscillator indices to infinite order, using the following identity,

$$\sum_{\nu_x=0}^{\infty} |\tilde\varphi_{\nu_x}(0)|^2\, e^{-\tau\hbar\nu_x\omega_x} = \frac{1}{\sqrt{4\pi}l_x}\sqrt{\frac{e^{\hbar\omega_x\tau}}{\sinh(\hbar\omega_x\tau)}}. \tag{S18}$$

This expression follows from the expansion of the density matrix of a single particle in a harmonic oscillator potential, at temperature $1/\tau$ [12, 14].

By combining Eqs. (S15, S16, S17, S18), we can express the vacuum $T$-matrix in the analytic form

$$\frac{1}{\mathcal{T}(\omega,q)} = \frac{m}{4\pi\hbar^2}\left(\frac{1}{a} + \frac{1}{\sqrt{4\pi}\,l_xl_z}\mathcal{W}\left(\frac{\hbar\omega + i0^+ - \frac{\hbar^2q^2}{4m}}{\hbar\sqrt{\omega_x\omega_z}}\right)\right), \tag{S19}$$

where the function $\mathcal{W}$ is regular, and it is defined as

$$\begin{aligned}\mathcal{W}(\alpha) = &\int_0^\infty \frac{dx}{\sqrt{x}}\left(e^{\alpha x}\left[\sqrt{\frac{e^{(\eta+1/\eta)x}}{\sinh(\eta x)\,\sinh(x/\eta)}} - 4\pi l_xl_z \sum_{\nu_x=0}^{\tilde\nu_x}\sum_{\nu_z=0}^{\tilde\nu_z} |\tilde\varphi_{\nu_x}(0)|^2\, |\tilde\varphi_{\nu_z}(0)|^2\, e^{-x(\nu_x\eta+\nu_z/\eta)}\right] - \frac{1}{x}\right)\\ &+ i\sqrt{\pi}\sum_{\nu_x=0}^{\tilde\nu_x}\sum_{\nu_z=0}^{\tilde\nu_z} 4\pi l_xl_z\, |\tilde\varphi_{\nu_x}(0)|^2\, |\tilde\varphi_{\nu_z}(0)|^2 \frac{1}{\sqrt{\alpha + i0^+ - (\nu_x\eta + \nu_z/\eta)}},\end{aligned} \tag{S20}$$

with the parameter $\eta = \sqrt{\omega_x/\omega_z}$ characterizing the ellipticity of the confining potential. $\mathcal{W}$ incorporates the effects of confinement on the interaction [7], and renormalizes the $T$-matrix through Eq. (S19). In case of circularly symmetric waveguides, $\omega_x = \omega_z$, Eqs. (S19, S20) agree with earlier results of Refs. 3 and 15.

Two-particle bound states are defined as the poles of the vacuum $T$-matrix in Eq. (S19). Their energy $E_B$ is related to the scattering length as

$$-\frac{\sqrt{4\pi l_x l_z}}{a} = \mathcal{W}\left(\frac{E_B}{\hbar\sqrt{\omega_x\omega_z}}\right). \tag{S21}$$

Although in three dimensional systems, bound states appear only on the BEC side of the Feshbach resonance [16], quasi-one dimensional systems always exhibit a bound state, irrespective of the sign of the scattering length [3–5].

## IV. MANY-BODY PROBLEM: REGULARIZATION OF THE BCS ENERGY

In this section, we show that the BCS mean-field energy of the elliptical constriction Eq. (S8) is free of divergences, when expressed in terms of the scattering length $a$ or the bound state energy $E_B$. As a first step, we identify the singular part of the sum in Eq. (S8) by expanding the Bogoliubov energies in terms of the superconducting order parameter, and show that this UV divergence is canceled by Eq. (S15). In three dimensional gases, the singularity of the BCS mean-field energy is associated with the second order term in the expansion of the Bogoliubov energies, and all higher order terms give a finite contribution [16, 17]. This is also the case in the quasi-two dimensional confined system, as we will show by expanding $E_{\mathbf{n},q}$ in terms of the order paramters $\Delta_{\mathbf{N}}$ within perturbation theory [18].

At large momenta and channel indices, the pairing gap becomes negligible as compared to the kinetic energy, $\xi_{\mathbf{n},\mathbf{q}} \gg \sum_{\mathbf{n}_2} |\tilde{\Delta}_{\mathbf{n},\mathbf{n}_2}|$, the anomalous terms of the Hamiltonian Eq. (S6) can thus be treated as perturbation, $\mathbf{H}_{MF}(q) = \mathbf{H}_0(q) + \delta\mathbf{H}$, with

$$\mathbf{H}_0 = \begin{pmatrix} \boldsymbol{\xi}(q) & 0 \\ 0 & -\boldsymbol{\xi}(q) \end{pmatrix},$$
$$\delta\mathbf{H} = \begin{pmatrix} 0 & \tilde{\boldsymbol{\Delta}} \\ \tilde{\boldsymbol{\Delta}}^\dagger & 0 \end{pmatrix}.$$

Since $\delta\mathbf{H}$ contains only anomalous terms, odd orders in perturbation theory automatically become zero. The lowest order term in the expansion $E_{\mathbf{n},q} = E^{(0)}_{\mathbf{n},q} + \delta E^{(2)}_{\mathbf{n},q} + \delta E^{(4)}_{\mathbf{n},q} + \mathcal{O}\left(\|\boldsymbol{\Delta}\|^6\right)$ is simply given by the normal state spectrum, $E^{(0)}_{\mathbf{n},q} = \langle \mathbf{n}\uparrow|\mathbf{H}_0|\mathbf{n}\uparrow\rangle = \xi_{\mathbf{n},q}$, that is exactly canceled in Eq. (S8). The second order term has, however, a singular contribution to mean-field energy,

$$\delta E^{(2)}_{\mathbf{n},q} = \sum_{\mathbf{m}} \frac{|\langle \mathbf{m}\downarrow|\delta\mathbf{H}|\mathbf{n}\uparrow\rangle|^2}{\langle \mathbf{n}\uparrow|\mathbf{H}_0|\mathbf{n}\uparrow\rangle - \langle \mathbf{m}\uparrow|\mathbf{H}_0|\mathbf{m}\uparrow\rangle} = \sum_{\mathbf{m}} \frac{\left|\sum_{\mathbf{N}} \Delta_{\mathbf{N}} (V^\dagger_{\mathbf{N}})^{\mathbf{m},\mathbf{n}}\right|^2}{\xi_{\mathbf{n},q} + \xi_{\mathbf{m},q}}. \tag{S22}$$

As we show in the second part of this section, this singularity is canceled by the regularization of the coupling constant $g$. Finally, the contribution of the fourth order term

$$\delta E^{(4)}_{\mathbf{n},q} = \sum_{\mathbf{m}_1,\mathbf{m}_2\neq\mathbf{n},\mathbf{m}_3} \frac{\langle \mathbf{n}\uparrow|\delta\mathbf{H}|\mathbf{m}_1\downarrow\rangle\langle \mathbf{m}_1\uparrow|\delta\mathbf{H}|\mathbf{m}_2\uparrow\rangle\langle \mathbf{m}_2\uparrow|\delta\mathbf{H}|\mathbf{m}_3\downarrow\rangle\langle \mathbf{m}_3\uparrow|\delta\mathbf{H}|\mathbf{n}\uparrow\rangle}{(\xi_{\mathbf{n}}+\xi_{\mathbf{m}_1})(\xi_{\mathbf{m}_1}+\xi_{\mathbf{m}_2})(\xi_{\mathbf{m}_2}+\xi_{\mathbf{n}})} - \left(\sum_{\mathbf{m}} \frac{|\langle \mathbf{m}\downarrow|\delta\mathbf{H}|\mathbf{n}\uparrow\rangle|^2}{\xi_{\mathbf{n},q}+\xi_{\mathbf{m},q}}\right)^2 \tag{S23}$$

is regularized, similarly to all higher order terms. The somewhat technical derivation of this result is given in Ref. 19.

We remove the singularity of Eq. (S22), by expressing the bare coupling $g$ in terms of the $T$-matrix of the confined system in Eq. (S12). In the center of mass channel $\mathbf{N}$, the energy $\omega$ of incoming particles is simply shifted by $\mathbf{N}\cdot\boldsymbol{\omega}$ (see Eq. (S11)),

$$\frac{1}{g} = \frac{1}{\mathcal{T}(\omega - \mathbf{N}\cdot\boldsymbol{\omega}, q)} + \sum_{\boldsymbol{\nu}} |\tilde{\varphi}_{\boldsymbol{\nu}}(0)|^2\, \Pi^{(0)}_{\boldsymbol{\nu}}(\omega - \mathbf{N}\cdot\boldsymbol{\omega}, q)$$
$$= \frac{1}{\mathcal{T}(\omega - \mathbf{N}\cdot\boldsymbol{\omega}, q)} + \sum_{\boldsymbol{\nu}} |\tilde{\varphi}_{\boldsymbol{\nu}}(0)|^2\, \Pi^{(0)}_{\mathbf{N}+\boldsymbol{\nu}}(\omega, q)$$

By inserting a full basis $1 = \sum_{\mathbf{n}_1,\mathbf{n}_2} |\mathbf{n}_1,\mathbf{n}_2\rangle\langle\mathbf{n}_1,\mathbf{n}_2|$, we can rewrite $g$ as

$$\frac{1}{g} = \frac{1}{\mathcal{T}(\omega - \mathbf{N}\cdot\boldsymbol{\omega}, q)} + \sum_{\boldsymbol{\nu},\mathbf{n}_1,\mathbf{n}_2} \left(\langle \mathbf{N},\boldsymbol{\nu}|\mathbf{n}_1,\mathbf{n}_2\rangle\tilde{\varphi}_{\boldsymbol{\nu}}(0)\right)\left(\tilde{\varphi}_{\boldsymbol{\nu}}(0)\langle \mathbf{n}_1,\mathbf{n}_2|\mathbf{N},\boldsymbol{\nu}\rangle\right)\Pi^{(0)}_{\mathbf{N}+\boldsymbol{\nu}}(\omega, q).$$

We make use of the definition of the matrices $V_{\mathbf{N}}^{\mathbf{n}_1\mathbf{n}_2}$ above Eq. (S5) and that of the polarization operator in Eq. (S16), to rewrite the coupling as

$$\frac{1}{g}=\frac{1}{\mathcal{T}(\omega-\mathbf{N}\cdot\boldsymbol{\omega},q)}+\frac{1}{l_xL_yl_z}\sum_q\sum_{\mathbf{n}_1,\mathbf{n}_2}\frac{(V_{\mathbf{N}}^{\dagger})^{\mathbf{n}_1,\mathbf{n}_2}\,V_{\mathbf{N}}^{\mathbf{n}_1\mathbf{n}_2}}{\hbar\omega+i0^+-\left(\frac{\hbar^2q^2}{m}+\hbar(\mathbf{n}_1+\mathbf{n}_2)\cdot\boldsymbol{\omega}\right)}. \tag{S24}$$

Using this relation, we rewrite the second term in the mean-field energy $E_{MF}$ in Eq. (S8) as

$$\sum_{\mathbf{N}}\frac{|\Delta_{\mathbf{N}}|^2}{g}=\sum_{\mathbf{N}}\frac{|\Delta_{\mathbf{N}}|^2}{\mathcal{T}(\omega-\mathbf{N}\cdot\boldsymbol{\omega},q)}+\frac{1}{l_xL_yl_z}\sum_{\mathbf{n}_1,\mathbf{n}_2,q}\frac{\sum_{\mathbf{N}}\left|\Delta_{\mathbf{N}}(V_{\mathbf{N}}^{\dagger})^{\mathbf{n}_1\mathbf{n}_2}\right|^2}{\hbar\omega+i0^+-\left(\frac{\hbar^2q^2}{m}+\hbar(\mathbf{n}_1+\mathbf{n}_2)\cdot\boldsymbol{\omega}\right)}. \tag{S25}$$

This expression has the same asymptotic behavior in the $(q,\mathbf{n}_1,\mathbf{n}_2)\to\infty$ limit as the second order expansion of $\sum_{\mathbf{n},q}E_{\mathbf{n},q}$ in Eq. (S22). Therefore, it exactly cancels the singular part of mean-field energy, and we can combine Eqs. (S19 S8, S25), to rewrite $E_{MF}$ in the regularized form

$$\begin{aligned}\frac{E_{MF}}{L_y}=\int\frac{dq}{2\pi}&\left[\sum_{\mathbf{n}}(\xi_{\mathbf{n},q}-E_{\mathbf{n},q})-\sum_{\mathbf{n}_1,\mathbf{n}_2}\frac{\sum_{\mathbf{N}}\left|\Delta_{\mathbf{N}}(V_{\mathbf{N}}^{\dagger})^{\mathbf{n}_1\mathbf{n}_2}\right|^2}{\omega+i0^+-\left(\frac{\hbar^2q^2}{m}+\hbar(\mathbf{n}_1+\mathbf{n}_2)\cdot\boldsymbol{\omega}\right)}\right]\\&-\sum_{\mathbf{N}}\frac{|\Delta_{\mathbf{N}}|^2}{4\pi\sqrt{\omega_x\omega_z}}\left(\frac{1}{a}+\frac{1}{\sqrt{4\pi}\,l_xl_z}\mathcal{W}\left(\frac{\omega+i0^+-\mathbf{N}\cdot\boldsymbol{\omega}}{\sqrt{\omega_x\omega_z}}\right)\right),\end{aligned} \tag{S26}$$

with the function $\mathcal{W}$ defined in Eq. (S20). Note that in the last equation, the parameter $\omega$ is completely arbitrary, since the $\omega$ dependence of the two terms cancel.

Although Eq. (S26) allows for pairing within all transverse channels $\mathbf{N}$, only $\Delta_{\mathbf{N}=0}$ takes on non-zero value for the parameters of the experiment [20]. This allows for a further simplification of the mean-field energy. By choosing $\omega$ at the energy of the two-particle bound state in Eq. (S26), the second term vanishes due to Eq. (S21), and the mean-field energy becomes

$$\frac{E_{MF}}{L_y}=\int\frac{dq}{2\pi}\left[\sum_{\mathbf{n}}(\xi_{\mathbf{n},q}-E_{\mathbf{n},q})-\sum_{\mathbf{n}_1,\mathbf{n}_2}\frac{|\Delta_{\mathbf{0}}|^2\,|V_{\mathbf{0}}^{\mathbf{n}_1\mathbf{n}_2}|^2}{E_B-\left(\frac{\hbar^2q^2}{m}+\hbar(\mathbf{n}_1+\mathbf{n}_2)\cdot\boldsymbol{\omega}\right)}\right].$$

This expression is equivalent to Eq. (6) in the main text.

Furthermore, Eq. (S24) allows one to derive the dependence of the bound state energy on the bare coupling, as shown in Eq. (5). We choose the incoming energy at $E_B$, so that the first term in Eq. (S24) is zero, and we find

$$\frac{1}{g}=\frac{1}{l_xl_z}\frac{1}{L_y}\sum_q\sum_{\mathbf{n}_1,\mathbf{n}_2}\frac{|V_{\mathbf{0}}^{\mathbf{n}_1\mathbf{n}_2}|^2}{E_B-\left(\frac{\hbar^2q^2}{m}+\hbar(\mathbf{n}_1+\mathbf{n}_2)\cdot\boldsymbol{\omega}\right)}$$

in the $\mathbf{N}=0$ channel.

## V. TRANSPORT THROUGH THE CHANNEL

We determine the conductance and spin conductance of the quasi-one dimensional constriction within Landauer theory, by calculating its reflection and Andreev reflection coefficients. These can be obtained from the asymptotic behavior of scattering eigenstates of the constriction. To determine these states, one has to solve the spatially non-uniform Bogoliubov–de Gennes (BdG) equations, since the confinement frequencies $\omega_x(y)$ and $\omega_z(y)$, as well as the potential $V(y)$ and the superconducting order parameters $\Delta_{\mathbf{N}}(y)$ all change along the constriction. We do this by dividing the constriction into short intervals $(y_{i-1},y_i)$, in which the system's parameters can be approximated as constants, as shown in Fig. S2. We require furthermore that the wave functions of the eigenstates change smoothly at the interfaces between the intervals. In each interval, the scattering eigenstates of energy $\epsilon$ above the Fermi energy are described by the local BdG equation

$$\begin{pmatrix}\mathcal{H}_{0,i} & \Delta_i\\ \Delta_i^{\dagger} & -\mathcal{H}_{0,i}^*\end{pmatrix}\begin{pmatrix}u_i(x,z)\\ v_i(x,z)\end{pmatrix}e^{iqy}=\epsilon\begin{pmatrix}u_i(x,z)\\ v_i(x,z)\end{pmatrix}e^{iqy}, \tag{S27}$$

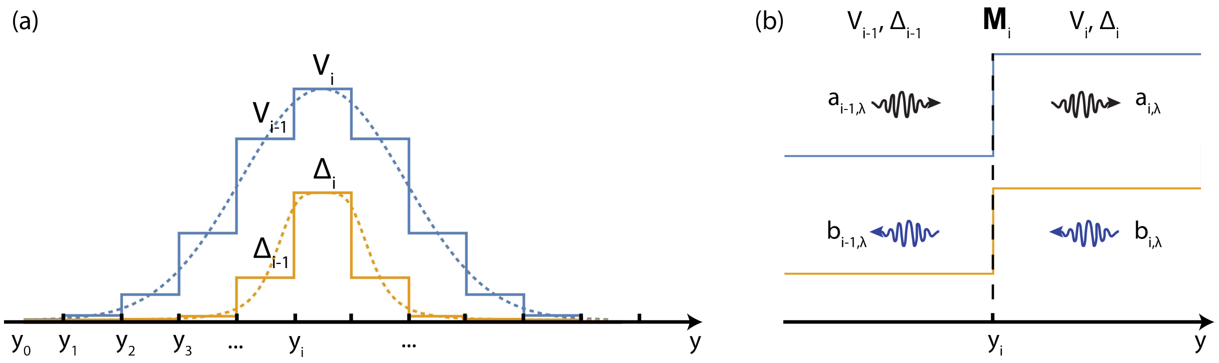


FIG. S2. Conductance calculation. (a) We divide the constriction into finite intervals, in which the potential $V(y)$ and the superconducting order parameters $\Delta_{\mathbf{N}}(y)$ are approximated as constants. (b) We derive the transfer matrix $\mathbf{M}_i$ by requiring the wave function to be continuous and differentiable at each interface $y_i$.

where the kinetic and anomalous terms in the Hamiltonian are given by

$$\mathcal{H}_{0,i}(x,z) = q^2/2m - \epsilon_{F,i} + \sum_{\mathbf{n}} \mathbf{n}\cdot\boldsymbol{\omega}_i \; |\mathbf{n}_i(x,z)\rangle\langle\mathbf{n}_i(x,z)|\,,$$

$$\Delta_i(x,z) = \sum_{\mathbf{n}_1\mathbf{n}_2} \Delta_{i,\mathbf{n}_1\mathbf{n}_2}\, |\mathbf{n}_{i,1}(x,z)\rangle\langle\mathbf{n}_{i,2}(x,z)|\,.$$

Here, the value of the local Fermi energy is given by $\epsilon_{F,i} = \mu - V_i - (\omega_{x,i} + \omega_{z,i})/2$, and the states $|\mathbf{n}_i(x,z)\rangle$ denote the transverse wave functions of the harmonic oscillator. We use the index $\lambda$ to label the modes corresponding to energy $\epsilon$,

$$|\Psi_i(x,z)\rangle \equiv \begin{pmatrix} u_i(x,z) \\ v_i(x,z) \end{pmatrix} = \sum_{\lambda} \left(a_{i\lambda} e^{iq_{i\lambda}y} + b_{i\lambda} e^{-iq_{i\lambda}y}\right) \sum_{\mathbf{n}} \begin{pmatrix} u_{i\lambda\mathbf{n}} \\ v_{i\lambda\mathbf{n}} \end{pmatrix} |\mathbf{n}_i(x,z)\rangle, \tag{S28}$$

with $a_{i\lambda}$ and $b_{i\lambda}$ denoting the amplitudes of left and right moving modes. Most of these modes are evanescent, and the $q_{i\lambda}$ wave vector is imaginary. We solve Eq. (S27), in order to determine the wave vectors. This leads to an eigenvalue equation for $q_{i\lambda}$ [21],

$$\frac{q_{i\lambda}^2}{2m} \begin{pmatrix} \mathbf{u}_{i\lambda} \\ \mathbf{v}_{i\lambda} \end{pmatrix} = \begin{pmatrix} \epsilon + \epsilon_{F,i} - \boldsymbol{\Omega}_i & -\boldsymbol{\Delta}_i \\ \boldsymbol{\Delta}_i^\dagger & -\epsilon + \epsilon_{F,i} - \boldsymbol{\Omega}_i \end{pmatrix} \begin{pmatrix} \mathbf{u}_{i\lambda} \\ \mathbf{v}_{i\lambda} \end{pmatrix}, \tag{S29}$$

where $\boldsymbol{\Omega}_{i,\mathbf{n}_1\mathbf{n}_2} \equiv \delta_{\mathbf{n}_1\mathbf{n}_2}\, \mathbf{n_1}\cdot\boldsymbol{\omega}_i$ denotes the harmonic oscillator energies, whereas $(\boldsymbol{\Delta}_i)_{\mathbf{n}_1\mathbf{n}_2} \equiv \Delta_{i,\mathbf{n}_1\mathbf{n}_2}$ stands for the matrix of superconducting order parameters. We also introduced the vectorial notations $(\mathbf{u}_{i\lambda})_{\mathbf{n}} \equiv u_{i\lambda\mathbf{n}}$ and $(\mathbf{v}_{i\lambda})_{\mathbf{n}} \equiv v_{i\lambda\mathbf{n}}$ for the Bogoliubov modes of the eigenstates. The transfer matrix at point $y_i$ describes the relation between the amplitudes on the two sides of the interface

$$\begin{pmatrix} \vec{a}_i \\ \vec{b}_i \end{pmatrix} = \mathbf{M}_i \begin{pmatrix} \vec{a}_{i-1} \\ \vec{b}_{i-1} \end{pmatrix}.$$

Here, we introduced the vectorial notation $(\vec{a}_i)_\lambda = a_{i\lambda}$ and $(\vec{b}_i)_\lambda = b_{i\lambda}$ for the amplitudes of the BdG states. $\mathbf{M}_i$ can be determined by requiring the continuity and differentiability of the wave function at $y_i$,

$$|\Psi_{i-1}(y_i)\rangle = |\Psi_i(y_i)\rangle,$$
$$\partial_y|\Psi_{i-1}(y_i)\rangle = \partial_y|\Psi_i(y_i)\rangle.$$

To determine the transfer matrix, we take the matrix elements of these equations with the transverse oscillator modes $\langle\mathbf{n}_i(x,z)|$, and make use of the expansion Eq. (S28) of the wave function, to get

$$\sum_{\lambda} \left(a_{i-1\lambda} e^{iq_{i-1\lambda}y_i} + b_{i-1\lambda} e^{-iq_{i-1\lambda}y_i}\right) \sum_{\mathbf{n}'} \langle\mathbf{n}_i|\mathbf{n}'_{i-1}\rangle \begin{pmatrix} u_{i-1\,\lambda\mathbf{n}'} \\ v_{i-1\,\lambda\mathbf{n}'} \end{pmatrix} = \sum_{\lambda} \left(a_{i\lambda} e^{iq_{i\lambda}y_i} + b_{i\lambda} e^{-iq_{i\lambda}y_i}\right) \begin{pmatrix} u_{i\lambda\mathbf{n}} \\ v_{i\lambda\mathbf{n}} \end{pmatrix},$$

$$\sum_{\lambda} q_{i-1\lambda} \left(a_{i-1\lambda} e^{iq_{i-1\lambda}y_i} - b_{i-1\lambda} e^{-iq_{i-1\lambda}y_i}\right) \sum_{\mathbf{n}'} \langle\mathbf{n}_i|\mathbf{n}'_{i-1}\rangle \begin{pmatrix} u_{i-1\,\lambda\mathbf{n}'} \\ v_{i-1\,\lambda\mathbf{n}'} \end{pmatrix} = \sum_{\lambda} q_{i\lambda} \left(a_{i\lambda} e^{iq_{i\lambda}y_i} - b_{i\lambda} e^{-iq_{i\lambda}y_i}\right) \begin{pmatrix} u_{i\lambda\mathbf{n}} \\ v_{i\lambda\mathbf{n}} \end{pmatrix}.$$

To simplify our notations, we rewrite these equations in a matrix form. We introduce the matrix $(\mathbf{W}_i)_{\mathbf{n}\mathbf{n}'} \equiv \langle \mathbf{n}_i | \mathbf{n}'_{i-1} \rangle$ that describes the unitary transformation from the harmonic oscillator basis in the interval $(y_{i-1}, y_i)$ to that of $(y_i, y_{i+1})$. A short calculation shows that the transfer matrix is given by,

$$\mathbf{M}_i = \frac{1}{2} \begin{pmatrix} e^{-i\vec{q}_i\, y_i} & -e^{-i\vec{q}_i\, y_i} \\ e^{i\vec{q}_i y_i} & e^{i\vec{q}_i y_i} \end{pmatrix} \begin{pmatrix} \mathbf{U}_i^{-1} \begin{pmatrix} \mathbf{W}_i & 0 \\ 0 & \mathbf{W}_i \end{pmatrix} \mathbf{U}_{i-1} & 0 \\ 0 & (\mathbf{U}_i \vec{q}_i)^{-1} \begin{pmatrix} \mathbf{W}_i & 0 \\ 0 & \mathbf{W}_i \end{pmatrix} \mathbf{U}_{i-1} \vec{q}_{i-1} \end{pmatrix} \begin{pmatrix} e^{i\vec{q}_i\, y_{i-1}} & e^{-i\vec{q}_i y_{i-1}} \\ -e^{i\vec{q}_i\, y_{i-1}} & e^{-i\vec{q}_i y_{i-1}} \end{pmatrix} \tag{S30}$$

where $\vec{q}_i$ denotes the matrix that has the momenta $q_{i\lambda}$ on its diagonal, and the matrix $\mathbf{U}_i$ contains the Bogoliubov coefficients

$$\mathbf{U}_i = \left( \begin{pmatrix} \mathbf{u}_{i,\lambda=1} \\ \mathbf{v}_{i,\lambda=1} \end{pmatrix}, \begin{pmatrix} \mathbf{u}_{i,\lambda=2} \\ \mathbf{v}_{i,\lambda=2} \end{pmatrix}, \begin{pmatrix} \mathbf{u}_{i,\lambda=3} \\ \mathbf{v}_{i,\lambda=3} \end{pmatrix}, \ \ldots \right).$$

One of the challenges in working with transfer matrices is that they are numerically unstable due to evanescent modes of the constriction. Although the transfer matrices of small intervals are well defined, that of the entire constriction, $\mathbf{M} = \prod_i \mathbf{M}_i$ contains elements that blow up or vanish exponentially with the system length $L_y$. We circumvent this difficulty by representing the scattering problem in terms of scattering matrices in each interval, which connect incoming states to outgoing ones,

$$\begin{pmatrix} \vec{b}_{i-1} \\ \vec{a}_i \end{pmatrix} = \mathbf{S}_i \begin{pmatrix} \vec{a}_{i-1} \\ \vec{b}_i \end{pmatrix}.$$

The transfer matrix and the scattering matrix are trivially related to each other [22]. However, the latter is free from the divergences associated with evanescent modes. We follow Ref. 23 to obtain the scattering matrix $\mathbf{S}$ of the constriction from those of individual intervals.

In the normal leads, the wave function of scattering states can be decomposed as

$$|\psi(\mathbf{r})\rangle = \sum_{\mathbf{n}} \left( e^{iq^p_{\mathbf{n}} y} \begin{pmatrix} \tilde{a}^p_{\mathbf{n}} \\ 0 \end{pmatrix} + e^{-iq^p_{\mathbf{n}} y} \begin{pmatrix} \tilde{b}^p_{\mathbf{n}} \\ 0 \end{pmatrix} \right) \frac{|\mathbf{n}(x,z)\rangle}{\sqrt{v^p_{\mathbf{n}}}} + \left( e^{iq^h_{\mathbf{n}} y} \begin{pmatrix} 0 \\ \tilde{a}^h_{\mathbf{n}} \end{pmatrix} + e^{-iq^h_{\mathbf{n}} y} \begin{pmatrix} 0 \\ \tilde{b}^h_{\mathbf{n}} \end{pmatrix} \right) \frac{|\mathbf{n}(x,z)\rangle}{\sqrt{v^h_{\mathbf{n}}}}, \tag{S31}$$

with the amplitudes $\tilde{a}^{p/h}_{\mathbf{n}}$ and $\tilde{b}^{p/h}_{\mathbf{n}}$ corresponding to right and left moving states in transverse channel $\mathbf{n}$. The momenta $q^{p/h}_{\mathbf{n}}$ are those of particle ($p$) and hole states ($h$) at energy $\epsilon$, and the associated group velocities are given by $v^{p/h}_{\mathbf{n}} = \hbar\, q^{p/h}_{\mathbf{n}}/m$. With the above normalization, all modes correspond to unit flux, and the scattering matrix of the constriction is unitary in this basis due to charge conservation [22].

The scattering matrix can be written in the usual representation in terms of reflection ($\mathbf{r}$) and transmission matrices ($\mathbf{t}$) as

$$\begin{pmatrix} \tilde{b}^p_L \\ \tilde{b}^h_L \\ \tilde{a}^p_R \\ \tilde{a}^h_R \end{pmatrix} = \mathbf{S} \begin{pmatrix} \tilde{a}^p_L \\ \tilde{a}^h_L \\ \tilde{b}^p_R \\ \tilde{b}^h_R \end{pmatrix} = \begin{pmatrix} \mathbf{r}_{pp} & \mathbf{r}_{ph} & \mathbf{t}'_{pp} & \mathbf{t}'_{ph} \\ \mathbf{r}_{hp} & \mathbf{r}_{hh} & \mathbf{t}'_{hp} & \mathbf{t}'_{hh} \\ \mathbf{t}_{pp} & \mathbf{t}_{ph} & \mathbf{r}'_{pp} & \mathbf{r}'_{ph} \\ \mathbf{t}_{hp} & \mathbf{t}_{hh} & \mathbf{r}'_{hp} & \mathbf{r}'_{hh} \end{pmatrix} \begin{pmatrix} \tilde{a}^p_L \\ \tilde{a}^h_L \\ \tilde{b}^p_R \\ \tilde{b}^h_R \end{pmatrix},$$

where the indices $L$ and $R$ denote states in the left and right leads, respectively. Although the elements of the scattering matrix depend on the energy of incoming particles $\epsilon$, we omitted the energy arguments for brevity. The zero bias charge and spin conductance of the constriction in Eq. (7) can be obtained from the reflection $\mathbf{r}_{pp}(\epsilon)$ and Andreev reflection coefficients $\mathbf{r}_{ph}(\epsilon)$ using the Landauer formula [22].

### A. Coefficients, $\mathbf{W}_i$

In order to calculate the transfer matrix $\mathbf{M}_i$ in Eq. (S30), we need to determine the unitary operator $\mathbf{W}_{\mathbf{n}\mathbf{n}'} = \langle \mathbf{n}_i | \mathbf{n}'_{i-1} \rangle = \langle n_{xi} | n'_{x\, i-1} \rangle \langle n_{zi} | n'_{z\, i-1} \rangle$, describing the change of harmonic oscillator basis between intervals $i$ and $i-1$. The harmonic oscillator eigenstates along $x$ are given by $|n_{xi}(x)\rangle = \hat{\varphi}_{n_x}(x/l_{xi})/\sqrt{l_{xi}}$, with the Hermite function

$$\hat{\varphi}_n(\tilde{x}) = \frac{1}{\sqrt{2^n\, n! \sqrt{\pi}}} e^{-\tilde{x}^2/2}\, H_n(\tilde{x}),$$

and a similar expression holds in case of the $z$ direction. We make use of the following identity of the Hermite polynomials [24]

$$H_n(\gamma\tilde{x}) = \sum_{l=0}^{\lfloor n/2 \rfloor} \gamma^{n-2l}(\gamma^2-1)^l \binom{n}{2l} \frac{(2l)!}{l!} H_{n-2l}(\tilde{x}),$$

to show that the matrix elements are given by

$$\langle n_{xi}|n'_{x\,i-1}\rangle = \sqrt{\gamma_{xi}}\,\alpha_{xi} \sum_{l=0}^{\lfloor n/2 \rfloor} \sum_{l'=0}^{\lfloor n\prime/2 \rfloor} \delta_{n-2l,n'-2l'}\, \alpha_{xi}^{n-2l}\beta_{xi}^{n'-2l'}\,(\alpha_{xi}^2-1)^l(\beta_{xi}^2-1)^{l'} \binom{n}{2l}\binom{n'}{2l'} \sqrt{\frac{(n-2l)!\,(n'-2l')!}{2^{2l+2l'}\,n!\,n'!}},$$

with $\alpha_{xi} \equiv \sqrt{2/(1+\gamma_{xi}^2)}$, $\beta_{xi} \equiv \alpha_{xi}\gamma_{xi}$, and $\gamma_{xi} \equiv l_{x\,i-1}/l_{xi} = \sqrt{\omega_{xi}/\omega_{x\,i-1}}$. A similar equation holds for $\langle n_{zi}|n'_{z\,i-1}\rangle$, from which $\mathbf{W_{nn'}}$ can be determined.

## VI. DYNAMICS OF SUPERCONDUCTING ORDER PARAMETER BEYOND MEAN-FIELD

In the main text we used a simple mean-field model of the superconductivity in the constriction. We now analyze fluctuations of the superconducting order parameter which arise due to a finite size of the superconducting island and its coupling to the reservoirs of normal fermions. To understand the role of phase fluctuations on the transport processes, we estimate the fluctuations of the superconducting phase $\varphi$ during the timescale $\tau$ of Andreev reflections. We use an effective impedance model to describe dynamics of the phase [25–27]. This model adopts a simple Gaussian description of phase fluctuations and requires specifying a frequency dependent impedance of the environment, which will be presented in the framework of a resistor-capacitor model. From the Gaussian nature of phase fluctuations we have

$$\langle e^{i(\varphi(\tau)-\varphi(0))}\rangle = e^{-\frac{1}{2}\left\langle(\varphi(\tau)-\varphi(0))^2\right\rangle}. \tag{S32}$$

For numerical estimates, it will be more convenient to work with the phase variation averaged over time $\tau$

$$\overline{\mathrm{Var}^2}\varphi_\tau \equiv \frac{1}{\tau}\int_0^\tau dt\,\langle(\varphi(t)-\varphi(0))^2\rangle. \tag{S33}$$

One can use $\overline{\mathrm{Var}^2}\varphi_\tau$ to obtain phase fluctuations $\langle(\varphi(\tau)-\varphi(0))^2\rangle = \partial_\tau(\tau\,\overline{\mathrm{Var}^2}\varphi_\tau)$. We express fluctuations in terms of the spectral power density

$$S_{\varphi\varphi}(\nu) = \int_0^\infty dt\, e^{2\pi i\,\nu t}\langle\varphi(t)\varphi(0)\rangle,$$

at frequency $\nu$. Making use of the symmetry $S_{\varphi\varphi}(\nu) = S_{\varphi\varphi}(-\nu)$, the fluctuations can be written in the form

$$\overline{\mathrm{Var}^2}\varphi_\tau = 4\int_0^\infty d\nu\, S_{\varphi\varphi}(\nu)\,\overline{\zeta}_\tau(\nu), \tag{S34}$$

with the kernel $\overline{\zeta}_\tau(\nu) = 1 - \frac{\sin(2\pi\nu\tau)}{2\pi\nu\tau}$, that vanishes as $\overline{\zeta}_\tau(\nu) \simeq \frac{2\pi^2}{3}(\nu\tau)^2$ at small frequencies $\nu \lesssim 1/(2\tau)$, thus providing a low frequency cutoff. At higher frequencies, $\overline{\zeta}_\tau(\nu) \simeq 1$.

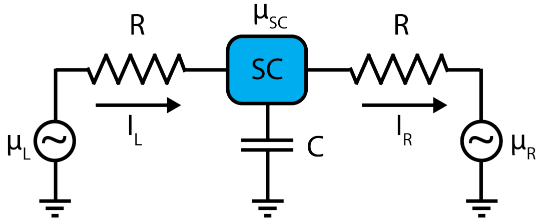


FIG. S3. Resistance capacitor model of phase fluctuations in the superconducting constriction.

To analyze the dynamics of phase fluctuations in a superconducting constriction, we use an effective resistor-capacitor model, shown in Fig. S3 [25–27]. The superconducting region is coupled to the leads through effective resistors $R = 1/(2G_A)$, where $G_A$ is the Andreev conductance of the constriction. The thermal Johnson–Nyquist noise associated with the leads is indicated by the $\mu_{L/R}$ voltage sources. The quantum capacitance $C_Q$ of the constriction arises from the energy cost of adding $\delta N$ atoms to the superconducting region, leading to a shift of its chemical potential

$$\mu_{sc} = \mu_{sc}^{(0)} + \frac{\delta N}{C_Q},$$

and the constant $\mu_{sc}^{(0)}$ denotes the time averaged equilibrium value of the chemical potential of the superconducting region. The physical motivation for Fig. S3 comes from the observation that it reproduces the semiclassical equations of motion for the current across the constriction. The current through the left and right superconducting interface are given by

$$I_L = \frac{\mu_{sc} - \mu_L}{R},$$
$$I_R = \frac{\mu_R - \mu_{sc}}{R},$$

and charge conservation in the superconducting region gives

$$\partial_t \, \delta N = I_L - I_R.$$

The spectral density of the Johnson–Nyquist noise of the chemical potential $\mu_{sc}$ at frequency $\nu$ is given by [28]

$$S_{\mu\mu}(\nu) = 4\, h\nu \, \mathrm{Re} Z(\nu) \, \left(\eta^{qm}(\nu) + \eta^{th}(\nu)\right), \tag{S35}$$

where $Z$ denotes the complex impedance $Z(\nu) = R/(1+i\nu/\nu_L)$ of the circuit between the constriction and the ground, with a relaxation frequency $\nu_L = (4\pi\, R\, C_Q)^{-1}$. Note that Eq. (S35) incorporates Johnson noise from both reservoirs, that are assumed to be independent. The frequency dependent factors

$$\eta^{qm}(\nu) = 1/2, \qquad \eta^{th}(\nu) = \frac{1/2}{e^{h\nu/k_B T} - 1} \tag{S36}$$

denote the noise contribution due to quantum and thermal fluctuations, respectively, as given by the fluctuation-dissipation theorem [28]. At small frequencies, $\nu \ll \nu_{th} \equiv k_B T/h$, thermal fluctuations dominate, $\eta_{th}(\nu) \sim \frac{k_B T}{2h\nu}$, leading to the Johnson–Nyquist noise formula of classical systems [29]. In the opposite limit, at high frequencies, thermal fluctuations vanish and the noise is dominated by quantum fluctuations.

Fluctuations of the phase $\varphi$ of the superconducting region are related to chemical potential fluctuations in the leads by the Josephson relation [17]

$$\hbar\, \partial_t \varphi = 2\, \mu_{sc}, \tag{S37}$$

which determines the spectral density

$$S_{\varphi\varphi}(\nu) = \left(\frac{2}{h\nu}\right)^2 S_{\mu\mu}(\nu). \tag{S38}$$

$S_{\varphi\varphi}$ can be determined by combining Eqs. (S35) and (S38),

$$S_{\varphi\varphi}(\nu) = \frac{8}{h\nu} \, \left(\eta^{qm}(\nu) + \eta^{th}(\nu)\right) \, \frac{R}{1 + \left(\frac{\nu}{\nu_L}\right)^2}.$$

Although the spectral power density is singular at small frequencies, its divergence is canceled in Eq. (S34) by the low frequency cut-off of the kernel $\overline{\zeta}_\tau(\nu) \sim (\nu\tau)^2$ at frequencies $\nu \lesssim \tau^{-1}$.

To estimate the growth of phase fluctuations with the time $\tau$, we first consider the system at zero temperature, where only quantum fluctuations contribute to Eq. (S34),

$$\overline{\mathrm{Var}^2 \varphi_\tau}^{qm} = \frac{16R}{h} \int_0^\infty \frac{d\nu}{\nu} \, \frac{\overline{\zeta}_\tau(\nu)}{1 + \left(\frac{\nu}{\nu_L}\right)^2}. \tag{S39}$$

At long times, $\tau \gg \nu_L^{-1}$, the integral in the last equation is dominated by the frequency range $(2\tau)^{-1} < \nu < \nu_L$, where

$$\overline{\mathrm{Var}^2 \varphi_{\tau \gg \nu_L^{-1}}}^{qm} \simeq \frac{16R}{h} \int_{\frac{1}{\tau}}^{\nu_L} \frac{d\nu}{\nu} \sim \frac{R}{h} \log(\tau\, \nu_L), \tag{S40}$$

which indicates that phase correlations $\langle e^{i\,\varphi(\tau)}\, e^{-i\,\varphi(0)} \rangle$ decay algebraically in time. In the opposite, short time limit, we can make use of the quadratic low frequency dependence of $\bar{\zeta}_\tau(\nu)$ below Eq. (S34). The integral is dominated by the same frequency range,

$$\overline{\mathrm{Var}^2 \varphi_{\tau \ll \nu_L^{-1}}}^{qm} \simeq \frac{32\pi^2}{3} \frac{R}{h} (\tau \nu_L)^2 \int_{\nu_L}^{\frac{1}{\tau}} \frac{d\nu}{\nu} \sim \frac{R}{h} (\tau\, \nu_L)^2 \log\left(\frac{1}{\tau \nu_L}\right). \tag{S41}$$

At finite temperatures, the low frequency fluctuations are dominated by thermal effects. Making use of the approximation $\eta^{th}(\nu \lesssim \nu_{th}) \sim \nu_{th}/\nu$, phase fluctuations in Eq. (S34) can be approximated as

$$\overline{\mathrm{Var}^2 \varphi_\tau}^{th} \simeq \frac{16R}{h} \nu_{th} \int_0^{\nu_{th}} \frac{d\nu}{\nu^2} \frac{\bar{\zeta}_\tau(\nu)}{1 + \left(\frac{\nu}{\nu_L}\right)^2}.$$

A simple calculation shows that thermal phase fluctuations grow linearly at long times

$$\overline{\mathrm{Var}^2 \varphi_{\tau \gg \nu_L^{-1}, \nu_{th}^{-1}}}^{th} \sim \frac{R}{h} (\tau\, \nu_{th}), \tag{S42}$$

which indicates phase diffusion. This is in accordance with our expectations that a mesoscopic superconducting region should have exponentially decaying temporal correlations with the timescale set by the temperature. The last equation also shows that thermal fluctuations dominate quantum effects, Eq. (S40) in the long time limit. At short times, on the other hand, thermal fluctuations are quadratic in $\tau$

$$\overline{\mathrm{Var}^2 \varphi_{\tau \ll \nu_L^{-1}, \nu_{th}^{-1}}}^{th} \sim \frac{R}{h} (\tau^2\, \nu_{th} \nu_L), \tag{S43}$$

they are thus of similar order as quantum fluctuations, Eq. (S41).

It is instructive to estimate the strength of the fluctuations over the time scale $\tau$ it takes to accommodate a Cooper pair in the process of Andreev reflection. We will use estimates of the relevant time and frequency scales $\tau$, $\nu_L$ and $\nu_{th}$ from the experimental parameters of Ref. 20. The width of the superconducting-normal interface is of the order of the superconducting correlation length $\xi$, thus the time scale of Andreev processes is given by

$$\tau = \frac{\xi}{v_s},$$

where $v_s$ is the superflow velocity of the condensate. $v_s$ can be obtained by considering the supercurrent through the constriction

$$I_s = \frac{\Delta\mu}{R} = n_0 v_s, \tag{S44}$$

where $\Delta\mu = (\mu_L - \mu_R)/2$ denotes the chemical potential bias. $\mu_L$ and $\mu_R$ are the chemical potentials of the left and right leads respectively.

We determine the resonance frequency $\nu_L$ of the resistor-capacitor model by estimating the quantum capacitance $C_Q$ of the constriction. $C_Q$ is related to the energy cost of adding extra atoms to the superconductor, and it is given by

$$\frac{1}{C_Q} = \frac{\partial^2 E_{sc}}{\partial N^2},$$

where $E$ denotes the energy of the superconducting region. To estimate the quantum capacitance, we assume that this region of length $L_0$ is uniform, with a one-dimensional density $n_0 = N/L_0$. Since the chemical potential is given by

$$\mu = \frac{\partial E_{sc}}{\partial N} = \frac{1}{L_0} \frac{\partial E_{sc}}{\partial n_0},$$

the quantum capacitance can be estimated as

$$\frac{1}{C_Q} = \frac{\partial \mu}{\partial N} = \frac{1}{L_0} \frac{1}{\frac{\partial n_0}{\partial \mu}}.$$

Assuming for the moment that the constriction is in the normal phase, the density is $n_0 = 4/\lambda_F$, with $\lambda_F$ denoting the Fermi wavelength. The quantum capacitance is thus given by

$$\frac{1}{C_Q} \sim \frac{\epsilon_F}{2} \frac{\lambda_F}{L_0}, \tag{S45}$$

where $\epsilon_F$ is the Fermi energy. In case when the channel is superconducting, we cannot give such a simple analytical formula for $C_Q$. However, we checked numerically, that its value changes only slightly even in the presence of a pairing gap as large as $\Delta \sim \epsilon_F$. We therefore use the estimate in Eq. (S45) in the following.

We estimate the phase fluctuations in the strongly interacting regime, where the transport is dominated by Andreev processes. In this regime, the superconducting gap is of the order of the Fermi energy $\Delta \sim \epsilon_F$, as we discuss in the main text. We assume an Andreev conductance of $G_A = 4/h$, the resistance in the model is thus $R = h/8$. We estimate the correlation length as $\xi \sim \frac{\hbar v_F}{\Delta} = \frac{\epsilon_F}{\Delta} \frac{\lambda_F}{\pi}$, with $v_F$ denoting the Fermi velocity. Furthermore, we assume a typical chemical potential bias of $\Delta\mu = 0.1\,\epsilon_F$ in Eq. (S44), leading to a low frequency cut-off of $\tau^{-1} = 0.45\,\epsilon_F/h$ in Eq. (S34). We use Eq. (S45) to estimate the resonance frequency of the resistor-capacitor circuit, $\nu_L = (4\pi\, R C_Q)^{-1} = 0.03\,\epsilon_F/h$. The temperature of the measurement Ref. 20 leads to the frequency $\nu_{th} = k_B T/h = 0.15\,\epsilon_F/h$. As these frequency scales are much smaller than $\tau^{-1}$, phase fluctuations are dominated by quantum effects. Using these parameters, we estimate the phase fluctuations Eq. (S34) as

$$\frac{\overline{\mathrm{Var}^2 \varphi_\tau}}{(2\pi)^2} \simeq 0.06.$$

The phase fluctuations are thus suppressed in this regime, justifying the use of the mean-field description presented in the main text.


[1] A. M. Fischer and M. M. Parish, Phys. Rev. A **88**, 023612 (2013).
[2] A. J. Leggett and S. Zhang, *The BEC-BCS Crossover and the Unitary Fermi-Gas* (Springer, 2011).
[3] M. Olshanii, Phys. Rev. Lett. **81**, 938 (1998).
[4] D. S. Petrov, M. Holzmann, and G. V. Shlyapnikov, Phys. Rev. Lett. **84**, 2551 (2000).
[5] D. S. Petrov and G. V. Shlyapnikov, Phys. Rev. A **64**, 012706 (2001).
[6] H. Moritz *et al.*, Phys. Rev. Lett. **94**, 210401 (2005).
[7] E. Haller, M. Gustavsson, M. J. Mark, J. G. Danzl, R. Hart, G. Pupillo, and H.-C. Nägerl, Science **325**, 1224 (2009).
[8] E. Haller *et al.*, Phys. Rev. Lett. **104**, 153203 (2010).
[9] B. Fröhlich *et al.*, Phys. Rev. Lett. **106**, 105301 (2011).
[10] A. T. Sommer *et al.*, Phys. Rev. Lett. **108**, 045302 (2012).
[11] S. Sala *et al.*, Phys. Rev. Lett. **110**, 203203 (2013).
[12] M. Kanasz-Nagy, E. A. Demler, and G. Zarnd, Phys. Rev. A **91**, 032704 (2015).
[13] V. Pietilä, D. Pekker, Y. Nishida, and E. Demler, Phys. Rev. A **85**, 023621 (2012).
[14] R. P. Feynman, *Statistical Mechanics: A Set Of Lectures* (Westview Press, 1998).
[15] W. Fu, Z. Yu, and X. Cui, Phys. Rev. A **85**, 012703 (2012).
[16] I. Bloch, J. Dalibard, and W. Zwerger, Rev. Mod. Phys. **80**, 885 (2008).
[17] M. Tinkham, *Introduction to Superconductivity*, (Dover Publications, 2004).
[18] To simplify our discussion, we assume a spin symmetric chemical potentials $\mu_\uparrow = \mu_\downarrow$. Systems with spin asymmetry can be treated analogously.
[19] The slowest decaying term in terms of momentum $q$ and channel index $\mathbf{n}$ in $\delta E^{(4)}_{\mathbf{n},q}$ is given by the second term in Eq. (S23). In order to investigate this term, we need to determine the asymptotic behavior of the matrix elements $V_{\mathbf{N}}^{\mathbf{n}_1\mathbf{n}_2}$ in the limit $\mathbf{n}_1, \mathbf{n}_2 \to \infty$. In a strongly confined system, pairing occurs only in the lowest few $\mathbf{N}$ channels, therefore we can assume that $\mathbf{N}$ is small. In this case, $V_{\mathbf{N}}^{\mathbf{n}_1\mathbf{n}_2}$ and $V_{\mathbf{0}}^{\mathbf{n}_1\mathbf{n}_2}$ are asymptotically of the same order. Furthermore, using the asymptotic formulas of harmonic oscillator wave functions, one can show that in the $\mathbf{n}_1, \mathbf{n}_2 \to \infty$ limit $V_{\mathbf{N}}^{\mathbf{n}_1\mathbf{n}_2}$ only takes on non-negligible values when $\mathbf{n}_1 \sim \mathbf{n}_2$. In this case, $V_{\mathbf{0}}^{\mathbf{n}\mathbf{n}} \sim 1/\sqrt{n_x n_z}$. Using this asymptotic form, we gain an upper limit on the asymptotic behavior of Eq. (S23), $E^{(4)}_{\mathbf{n},q} \sim n_x^{-2} n_z^{-2} \left(q^2/m + n_x\omega_x + n_z\omega_z\right)^{-2}$. The sum $\sum_{\mathbf{n},q} E^{(4)}_{\mathbf{n},q}$ thus gives a finite contribution to Eq. (S8). Furthermore, all higher order terms are regularized as well, since they contain even higher powers of $\xi^{-1}_{\mathbf{n},q}$ and $V_{\mathbf{N}}^{\mathbf{n}_1\mathbf{n}_2}$.

[20] S. Krinner *et al.*, arXiv:1511.05961.
[21] To make sure that the evanescent waves are indeed decaying in case of our right moving states, we take $E \to E + i0^+$.
[22] Y. V. Nazarov and Y. M. Blanter, *Quantum transport: Introduction to Nanoscience* (Cambridge University Press, 2009).
[23] P. W. Brouwer, M. Duckheim, A. Romito, and F. von Oppen, Phys. Rev. B **84**, 144526 (2011).
[24] M. Abramowitz and I. A. Stegun, *Handbook of Mathematical Functions with Formulas, Graphs, and Mathematical Tables* (United States Department of Commerce, National Bureau of Standards, 1964).
[25] S. M. Girvin, L. I. Glazman, M. Johnson, D. R. Penn and M. D. Stiles, Phys. Rev. Lett. **64**, 3183 (1990).
[26] H. Grabert and M. H. Devoret, *Single Charge Tunneling – Coulomb Blockade Phenomena in Nanostructures* (Springer, 1992).
[27] Y. Makhlin, G. Schön and A. Shnirman, Rev. Mod. Phys. **73**, 357 (2001).
[28] G. Schön and A. D. Zaikin, Phys. Rep. **198**, 237 (1990).
[29] H. Nyquist, Phys. Rev. **32**, 110 (1998).
